# Supplementary material for: Is Vanilla MLP in Neural Radiance Field Enough for Few-shot View Synthesis?
Source: arXiv:2403.06092 source file (2024-03-10)
Supplement: Supplementary file 1 [file X_suppl.tex]

\clearpage
\setcounter{page}{1}
\maketitlesupplementary

In Sec.~\ref{sec:Demonstration}, we provide a  detailed analysis of how mi-MLP works. Sec.~\ref{Experimental Details} introduces more experimental details, including datasets, metrics, implementation details, and methods used for comparison. We also report the results of using dropout to avoid overfitting in Sec.~\ref{Results of Using Dropout to Avoid Overfitting} and the extensions of mi-MLP to the task of 3D generation in Sec.~\ref{Extensions to 3D Generation}. More additional quantitative and qualitative results are provided in Sec.~\ref{Additional Results on Few-shot View Synthesis}. The limitations and future works are illustrated in Sec.~\ref{Limitations and Future Works}.

\section{How mi-MLP Works?}
\label{sec:Demonstration}
As illustrated in Sec.~\ref{sec:Per-layer Inputs Incorporation}, to mitigate the overfitting issue that usually occurs in few-shot view synthesis, we incorporate inputs into each layer of the MLP, which is denoted as:
\begin{equation}
  \centering \label{eq:suppl_equ_1}
  \textbf{\textit{f}}_i = \phi_i(\textbf{\textit{f}}_{i-1},\gamma_L(\textbf{\textit{x}})),\ \ \textbf{\textit{f}}_1 = \phi_1(\gamma_L(\textbf{\textit{x}})),
\end{equation}
where $\phi_i$ is the $i$-th ($i \ge 2$) layer of the MLP, $\textbf{\textit{f}}_i$ is the corresponding output feature, $\textbf{\textit{x}}$ is the input 5D coordinate and $\gamma_L(\textbf{\textit{x}})$ represents the endoded input embeddings obtained by Eq.~\ref{equ_2}.

Intuitively, during the early stage of training, with a common MLP initialization, Eq.~\ref{eq:suppl_equ_1} encourages a smaller amplitude of gradient for the shallower layer compared to that for the deeper layer, where the deeper layers (\ie, layers close to the outputs) are updated with large gradients while the shallower layers are updated with extremely small ones. \textbf{This implies that the model capacity is restricted at the start of training, which helps prevent the model from memorizing input views and thus avoids overfitting. However, as the number of network parameters remains unchanged, the total capacity of the model is preserved for more detailed rendering during the later stage of training.}

Specifically, assuming $\gamma_L(\textbf{\textit{x}})\in\mathbb{R}^{d_1 \times 1}$, $\textbf{\textit{f}}_i\in\mathbb{R}^{d_2 \times 1}$, the bias vector and weight matrix of $\phi_i$ are $\textbf{\textit{b}}_i\in\mathbb{R}^{d_2 \times 1}$ and $\textbf{\textit{w}}_i=(\textbf{\textit{w}}_i^1,\textbf{\textit{w}}_i^2,\dots,\textbf{\textit{w}}_i^{d_2})^T$ respectively, where $\textbf{\textit{w}}_i^j=(\textbf{\textit{w}}_i^{j0}\in\mathbb{R}^{1 \times d_1},\textbf{\textit{w}}_i^{j1}\in\mathbb{R}^{1 \times d_2})^T$. Thus Eq.~\ref{eq:suppl_equ_1} is equivalent to 
\begin{equation}
\centering \begin{split}
\label{eq:suppl_equ_2}
  \phi_i^j(\gamma_L(\textbf{\textit{x}})) = \epsilon \{\textbf{\textit{w}}_i^{j0} \cdot \gamma_L(\textbf{\textit{x}})+\textbf{\textit{w}}_i^{j1} \cdot \phi_{i-1}(\gamma_L(\textbf{\textit{x}}))+\textbf{\textit{b}}_i\},
\end{split}
\end{equation}
where $\phi_i^j$ is the $j$-th element of $\textbf{\textit{f}}_i$, $\epsilon$ denotes the activation fuction whose default setting is ReLU.

Assuming that the loss function is denoted as $\mathcal{L}$, then 
\begin{equation}
\begin{split}
    \centering \label{eq:suppl_equ_3}
    \Vert \frac{\partial \mathcal{L}}{\partial \textbf{\textit{w}}_i^{j0}} \Vert_1 = \Vert \frac{\partial \mathcal{L}}{\partial \phi_i^j} \cdot \frac{\partial \textbf{\textit{w}}_i^{j0} \cdot \gamma_L(\textbf{\textit{x}})}{\partial \textbf{\textit{w}}_i^{j0}} \Vert_1 = \Vert\frac{\partial \mathcal{L}}{\partial \phi_i^j}\Vert_1 \cdot \Vert \gamma_L(x) \Vert_1.
\end{split}
\end{equation}
\begin{equation}
\begin{split}
    \centering \label{eq:suppl_equ_4}
    \Vert \frac{\partial \mathcal{L}}{\partial \textbf{\textit{w}}_i^{j1}} \Vert_1 = \Vert \frac{\partial \mathcal{L}}{\partial \phi_i^j} \cdot \frac{\partial \textbf{\textit{w}}_i^{j1}  \cdot \phi_{i-1}}{\partial \textbf{\textit{w}}_i^{j1}} \Vert_1 = \Vert\frac{\partial \mathcal{L}}{\partial \phi_i^j}\Vert_1 \cdot \Vert \phi_{i-1} \Vert_1.
\end{split}
\end{equation}
\begin{equation}
\begin{split}
    \centering \label{eq:suppl_equ_5}
    \Vert \frac{\partial \mathcal{L}}{\partial \textbf{\textit{w}}_{i-1}^{j0}} \Vert_1 &= \Vert \frac{\partial \mathcal{L}}{\partial \phi_i^j} \cdot \frac{\partial \textbf{\textit{w}}_i^{j1} \cdot \phi_{i-1}}{\partial \phi_{i-1}^{j}} \cdot \frac{\partial \phi_{i-1}^{j}}{\partial \textbf{\textit{w}}_{i-1}^{j0}}\Vert_1 \\
    &= \Vert\frac{\partial \mathcal{L}}{\partial \phi_i^j}\Vert_1 \cdot \Vert \sum\textbf{\textit{w}}_i^{j1}\Vert_1 \cdot \Vert \gamma_L(x) \Vert_1.
\end{split}
\end{equation}
\begin{equation}
\begin{split}
    \centering \label{eq:suppl_equ_6}
    \Vert \frac{\partial \mathcal{L}}{\partial \textbf{\textit{w}}_{i-1}^{j1}} \Vert_1 &= \Vert \frac{\partial \mathcal{L}}{\partial \phi_i^j} \cdot \frac{\partial \textbf{\textit{w}}_i^{j1} \cdot \phi_{i-1}}{\partial \phi_{i-1}^{j}} \cdot \frac{\partial \phi_{i-1}^{j}}{\partial \textbf{\textit{w}}_{i-1}^{j1}}\Vert_1 \\
    &= \Vert\frac{\partial \mathcal{L}}{\partial \phi_i^j}\Vert_1 \cdot \Vert \sum\textbf{\textit{w}}_i^{j1}\Vert_1 \cdot \Vert \phi_{i-2} \Vert_1.
\end{split}
\end{equation}

As a result, 
\begin{equation}
\begin{split}
\centering \label{eq:suppl_equ_7}
  &\Vert \frac{\partial \mathcal{L}}{\partial \textbf{\textit{w}}_i} \Vert_1 / \Vert \frac{\partial \mathcal{L}}{\partial \textbf{\textit{w}}_{i-1}} \Vert_1 = \frac{1}{d_2}\sum_{j=1}^{d_2}\Vert \frac{\partial \mathcal{L}}{\partial \textbf{\textit{w}}_i^j} \Vert_1 / \Vert \frac{\partial \mathcal{L}}{\partial \textbf{\textit{w}}_{i-1}^j} \Vert_1 \\
  =& \frac{1}{d_2}\sum_{j=1}^{d_2}\Vert (\frac{\partial \mathcal{L}}{\partial \textbf{\textit{w}}_i^{j0}} \Vert_1 + \frac{\partial \mathcal{L}}{\partial \textbf{\textit{w}}_i^{j1}} \Vert_1) / (\Vert \frac{\partial \mathcal{L}}{\partial \textbf{\textit{w}}_{i-1}^{j0}} \Vert_1 + \Vert \frac{\partial \mathcal{L}}{\partial \textbf{\textit{w}}_{i-1}^{j1}} \Vert_1) \\
  =& \frac{1}{d_2}\sum_{j=1}^{d_2} \frac{\Vert \gamma_L(\textbf{\textit{x}}) \Vert_1 + \Vert \phi_{i-1}(\gamma_L(\textbf{\textit{x}})) \Vert_1}{\Vert \sum\textbf{\textit{w}}_i^{j1}\Vert_1\cdot\{\Vert \gamma_L(\textbf{\textit{x}}) \Vert_1 + \Vert \phi_{i-2}(\gamma_L(\textbf{\textit{x}})) \Vert_1\}}.
\end{split}
\end{equation}

Accordingly, during the early stage of training, if the MLP is initialized appropriately, where $\Vert \sum\textbf{\textit{w}}_i^{j1}\Vert_1\in(0,1]$ and $ \Vert \phi_{i-1}(\gamma_L(\textbf{\textit{x}})) \Vert_1 \approx \Vert \sum\textbf{\textit{w}}_i^{j1}\Vert_1 \cdot \Vert \phi_{i-2}(\gamma_L(\textbf{\textit{x}})) \Vert_1$, then $\Vert \frac{\partial \mathcal{L}}{\partial \textbf{\textit{w}}_i} \Vert_1 / \Vert \frac{\partial \mathcal{L}}{\partial \textbf{\textit{w}}_{i-1}} \Vert_1\ge 1$ holds true in a high probability.

In practice, we find that the default initialization provided by PyTorch for MLP can meet the requirements, where the weight matrix is uniformly initialized based on the dimension of the output feature. Specifically, taking $\textbf{\textit{w}}_i$ as an example, since the dimension of its output feature is $d_2$, each element of $\textbf{\textit{w}}_i$ is sampled from the following uniform distribution:
\begin{equation}
    \centering\label{eq:suppl_equ_8}
    \textbf{\textit{w}}_i \sim \mathcal{U}(-\frac{1}{\sqrt{d_2}},\frac{1}{\sqrt{d_2}}).
\end{equation}
On account that $\mathbb{E}[\textbf{\textit{w}}_i] = 0$, $\Vert \sum\textbf{\textit{w}}_i^{j1} \Vert_1 \approx \Vert d_2 \cdot \mathbb{E}[\textbf{\textit{w}}_i] \Vert_1 \approx 0$,
which demonstrates that $\Vert \sum\textbf{\textit{w}}_i^{j1}\Vert_1\in(0,1]$ holds.

Based on Eq.~\ref{eq:suppl_equ_2}, $\phi_{i-1}(\gamma_L(\textbf{\textit{x}}))=\epsilon(\textbf{\textit{w}}_{i-1}^0\cdot\gamma_L(\textbf{\textit{x}}) + \textbf{\textit{w}}_{i-1}^1\cdot\phi_{i-2}(\gamma_L(\textbf{\textit{x}})) + \textbf{\textit{b}}_i)$, where $\textbf{\textit{w}}_{i-1}^0\in\mathbb{R}^{d_2 \times d_1}$, $\textbf{\textit{w}}_{i-1}^1\in\mathbb{R}^{d_2 \times d_2}$. For an easier illustration and demonstration, we omit the influence of $\epsilon$, $\textbf{\textit{b}}_i$ and $\textbf{\textit{w}}_{i-1}^0$, thus 
\begin{equation}
    \centering
\begin{split}\label{eq:suppl_equ_9}
    \Vert \phi_{i-1}(\gamma_L(\textbf{\textit{x}})) \Vert_1\approx \Vert \textbf{\textit{w}}_{i-1}^1\cdot\phi_{i-2}(\gamma_L(\textbf{\textit{x}})) \Vert_1.
\end{split}
\end{equation}
Because each element in $\textbf{\textit{w}}_{i-1}^1$ is sampled from the same distribution, without loss of generality, we assume that $\sum w_i^{11} = \sum w_i^{21} = \dots = \sum w_i^{d_21}$. Consequently, 
\begin{equation}
    \centering
\begin{split}\label{eq:suppl_equ_10}
    &\Vert \textbf{\textit{w}}_{i-1}^1\cdot\phi_{i-2}(\gamma_L(\textbf{\textit{x}})) \Vert_1 = \Vert \sum\textbf{\textit{w}}_i^{j1}\Vert_1 \cdot \Vert \phi_{i-2}(\gamma_L(\textbf{\textit{x}})) \Vert_1.
\end{split}
\end{equation}

According to Eq.~\ref{eq:suppl_equ_9} and Eq.~\ref{eq:suppl_equ_10}, when the MLP is initialized by Eq.~\ref{eq:suppl_equ_8}, Eq.~\ref{eq:suppl_equ_7} can be conveted into the following formulation:
\begin{equation}
\begin{split}
\centering \label{eq:suppl_equ_11}
  &\Vert \frac{\partial \mathcal{L}}{\partial \textbf{\textit{w}}_i} \Vert_1 / \Vert \frac{\partial \mathcal{L}}{\partial \textbf{\textit{w}}_{i-1}} \Vert_1 \\
  =& \frac{1}{d_2}\sum_{j=1}^{d_2} \frac{\Vert \gamma_L(\textbf{\textit{x}}) \Vert_1 + \Vert \phi_{i-1}(\gamma_L(\textbf{\textit{x}})) \Vert_1}{\Vert \sum\textbf{\textit{w}}_i^{j1}\Vert_1\cdot\{\Vert \gamma_L(\textbf{\textit{x}}) \Vert_1 + \Vert \phi_{i-2}(\gamma_L(\textbf{\textit{x}})) \Vert_1\}}\\
  =& \frac{1}{d_2}\sum_{j=1}^{d_2} \frac{\Vert \gamma_L(\textbf{\textit{x}}) \Vert_1 + \Vert \sum\textbf{\textit{w}}_i^{j1}\Vert_1 \cdot \Vert \phi_{i-2}(\gamma_L(\textbf{\textit{x}}))}{\Vert \sum\textbf{\textit{w}}_i^{j1}\Vert_1\cdot\{\Vert \gamma_L(\textbf{\textit{x}}) \Vert_1 + \Vert \phi_{i-2}(\gamma_L(\textbf{\textit{x}})) \Vert_1\}}.
\end{split}
\end{equation}
Since $\Vert \sum\textbf{\textit{w}}_i^{j1}\Vert_1 \in (0,1]$, $\Vert \frac{\partial \mathcal{L}}{\partial \textbf{\textit{w}}_i} \Vert_1 / \Vert \frac{\partial \mathcal{L}}{\partial \textbf{\textit{w}}_{i-1}} \Vert_1 \ge 1$ holds, which demonstrates that with per-layer inputs incorporation, the amplitude of gradient of the shallow layer will be smaller than that of the deeper layer during the early stage of training.

\section{Experimental Details}
\label{Experimental Details}
\subsection{Datasets}
We perform experiments on a wide range of benchmarks, \ie, Blender~\cite{mildenhall2021nerf}, LLFF~\cite{mildenhall2019local}, and Shiny~\cite{wizadwongsa2021nex}, to demonstrate the effectiveness of our proposed method.

\paragraph{Blender.}
The Blender dataset is comprised of 8 object-centric $360^{\circ}$ inward-facing scenes, each containing 400 views. Following~\cite{jain2021putting}, when 8 input views are available, the images indexed $86,93,75,26,55,73,16,2$ are selected as the input views; when 4 input views are available, the images indexed $26,86,2,55$ are selected as the input views. For evaluation, the testing images are selected following~\cite{yang2023freenerf}. The resolution for both training views and testing views is $400\times400$.

\paragraph{LLFF.}
The LLFF dataset consists of 8 real-world forward-facing scenes. Following~\cite{niemeyer2022regnerf}, for each scene, every 8-th view is used as the holdout testing set and the training images are selected evenly from the remaining views. The resolution for both training views and testing views is $378\times504$. We report results when 3/6/9 input views are available.

\paragraph{Shiny.}
Similar to LLFF, the Shiny dataset also contains forward-facing scenes, while it is more complex due to its view-dependent effects such as reflection and refraction. We choose 6 scenes from the origional Shiny dataset and 2 scenes from the Shiny-extended dataset, where the resolution for each scene is $378\times504$.  The training and testing images are sampled following~\cite{niemeyer2022regnerf}.

\subsection{Metrics}
To measure the performance of our proposed method, we evaluate the quality of rendered novel views using Peak Signal-to-Noise Ratio (PSNR), Structural Similarity Index Measure (SSIM)~\cite{wang2004image}, and Learned Perceptual Image Patch Similarity (LPIPS)~\cite{zhang2018unreasonable}. Additionally, for an easier comparison, we also report the average score by calculating the geometric mean of $\text{MSE}=10^{-\text{PSNR}/10}$, $\sqrt{1-\text{SSIM}}$ and \text{LPIPS} following~\cite{niemeyer2022regnerf}.

\subsection{Implementation details}
We implement our approach using the nerf-pytorch codebase\footnote{\url{https://github.com/yenchenlin/nerf-pytorch}}, with vanilla NeRF as our baseline. For Blender, the values for $L_1$, $L_2$, and $L_3$ are set to be 2, 6, and 10 respectively; for LLFF and Shiny, the values for $L_1$, $L_2$, and $L_3$ are set to be 2, 8, and 10 respectively. For  $\mathcal\mathcal{L}_{\text{BR}}$, rays are sampled from extrapolated
image space where $p_x\in[-H/2, H+H/2]$ and $p_y\in[-W/2, W+W/2]$. For sampling annealing, we set $N_{\max}=256$, $N_{start}=16$, and $\eta = 100$. The Color Branch $C_{\theta}$ and Density Branch $D_{\theta}$ both have 8 layers with 256 neurons per layer. We apply 50K training iterations for Blender, while 200K training iterations for LLFF and Shiny. All experiments are performed on a single NVIDIA RTX 3090 GPU with a batch size of 1024. 

\subsection{Methods Used for Comparison}
To demonstrate the superiority of our proposed method, we compare it against several baselines, as well as prior-based and regularization-based methods. For baselines, we choose vanilla NeRF~\cite{mildenhall2021nerf}, Mip-NeRF~\cite{barron2021mip}, and Ref-NeRF~\cite{verbin2022ref}, which are all representative methods for novel view synthesis. For prior-based methods, following~\cite{yang2023freenerf}, we choose SRF~\cite{chibane2021stereo}, PixelNeRF~\cite{yu2021pixelnerf}, and MVSNeRF~\cite{chen2021mvsnerf}, where a large dataset is utilized to incorporate learned priors. We also report the fine-tuning results of these methods on LLFF and Shiny, which are able to obtain better performance. For regularization-based methods, we choose DietNeRF~\cite{jain2021putting}, InfoNeRF~\cite{kim2022infonerf}, RegNeRF~\cite{niemeyer2022regnerf}, MixNeRF~\cite{seo2023mixnerf}, as well as FreeNeRF~\cite{yang2023freenerf}, which are state-of-the-art methods for few-shot view synthesis to date. Notably, since the pre-trained network used in RegNeRF for appearance regularization is not provided, we only report the results of RegNeRF trained without it.

\section{Results of Using Dropout to Avoid Overfitting}
\label{Results of Using Dropout to Avoid Overfitting}
As explained in Sec.~\ref{sec:ablation}, we demonstrate the effectiveness of our mi-MLP by comparing it with the classical representative technique, \ie, Dropout~\cite{srivastava2014dropout}, which is used to avoid the overfitting problem.

Concretely, as shown in Fig.~\ref{fig:suppl_dropout}, for a testing scene randomly selected from the Blender dataset, a direct application of Dropout to the NeRF MLP leads to severe artifacts as well as unreasonable geometry. In contrast, our proposed method can achieve both photorealistic renderings and clear depth estimation. Quantitatively, as demonstrated in Tab.~\ref{tab:suppl_dropout}, Dropout obtains a comparable performance with DietNeRF~\cite{jain2021putting}, while a great performance improvement can be witnessed by using our mi-MLP.

\begin{figure}
    \centering
    \includegraphics[width=1\linewidth]{figs/suppl_dropout.png}
    \caption{The rendered novel views and estimated depth map by Dropout~\cite{srivastava2014dropout} and our proposed method respectively.}
    \label{fig:suppl_dropout}
\end{figure}

\begin{table}
    \resizebox{1\linewidth}{!}{\begin{tabular}{c|cccc}
    \toprule
    Method & PSNR$\uparrow$  & SSIM$\uparrow$  & LPIPS$\downarrow$ & Average$\downarrow$ \\
    \midrule
    DietNeRF~\cite{jain2021putting} & \cellcolor{orange!25}23.83 & \cellcolor{yellow!25}0.859 & \cellcolor{yellow!25}0.117 & \cellcolor{yellow!25}0.056 \\
    Dropout~\cite{srivastava2014dropout} & \cellcolor{yellow!25}23.79 & \cellcolor{orange!25}0.875 & \cellcolor{orange!25}0.108 & \cellcolor{orange!25}0.054 \\
    mi-MLP (Ours) & \cellcolor{red!25}25.50  & \cellcolor{red!25}0.887 & \cellcolor{red!25}0.087 & \cellcolor{red!25}0.043 \\
    \bottomrule
    \end{tabular}%}
    \caption{The quantitative results of DietNeRF~\cite{jain2021putting}, Dropout~\cite{srivastava2014dropout}, and our proposed mi-MLP respectively.
    }
    \label{tab:suppl_dropout}
\end{table}

\section{Extensions to 3D Generation}
\label{Extensions to 3D Generation}
As an important topic in computer vision and graphics, 3D generation can be viewed as an extreme case of few-shot view synthesis, where only one reference image or a textual description is available. To demonstrate the potential of our proposed method, we extend it to the task of Text-to-3D. Specifically, we take the public-available stable-dreamfusion\footnote{A reimplemented version of DreamFusion~\cite{poole2022dreamfusion} by Stable Diffusion} as an example, where we replace the network structure with our proposed mi-MLP.

As shown in Fig.~\ref{fig:hamburger}, combined with mi-MLP, the stable-dreamfusion is more robust to different textual descriptions, where reasonable results can be generated. In contrast, sometimes the original stable-dreamfusion falls into a degradation solution, generating nothing but pure colors. Such an observation shows that mi-MLP is beneficial to generating diverse 3D assets, which opens up a new direction for future research.

\begin{figure}
    \centering
    \begin{subfigure}[t]{1.0\linewidth}
         \centering
    \includegraphics[width=1\linewidth]{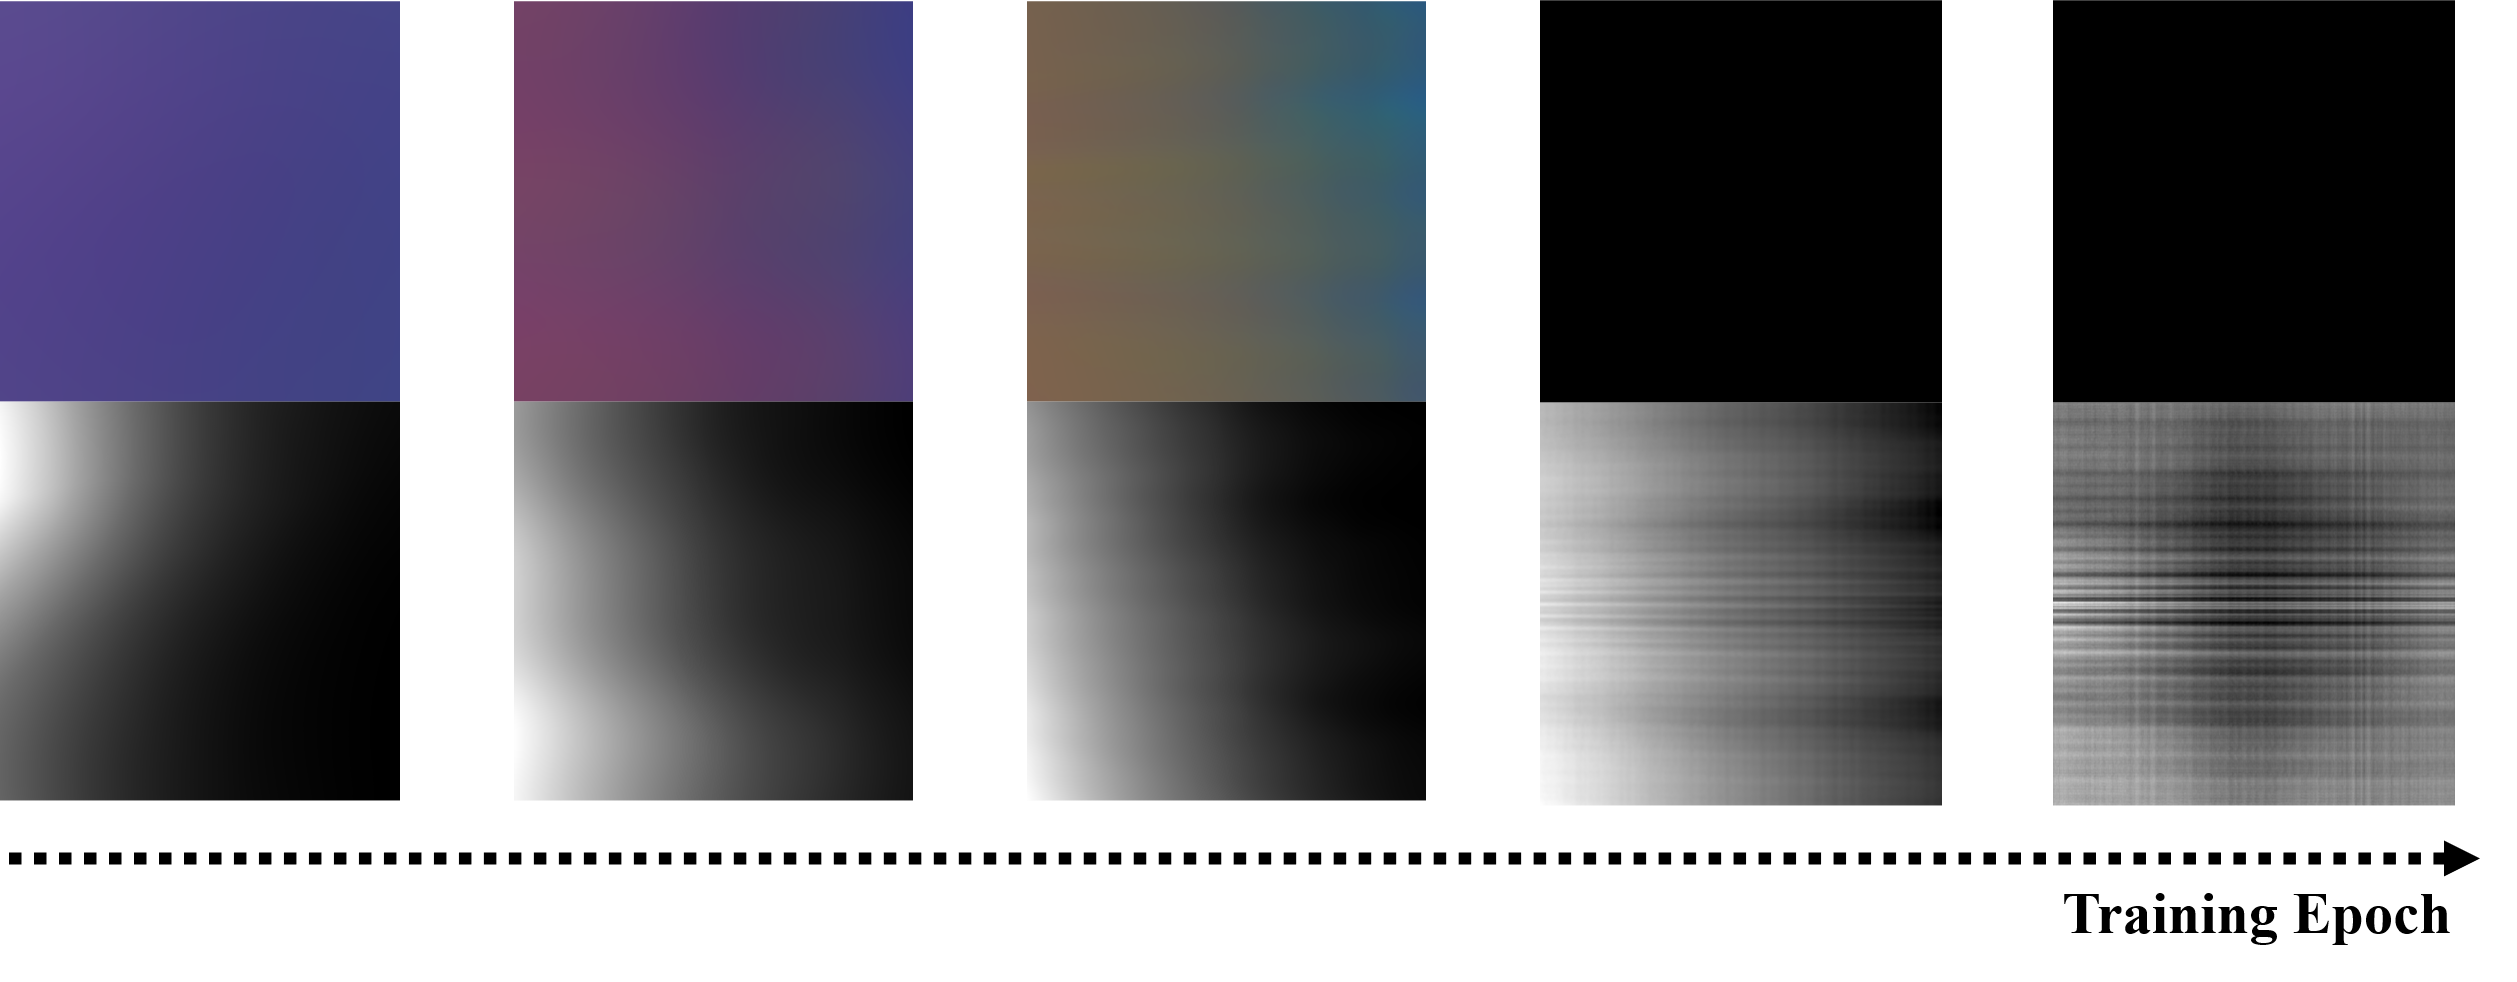}
    \caption{The training process of original stable-dreamfusion.}
    \end{subfigure}
    \begin{subfigure}[t]{1.0\linewidth}
         \centering
    \includegraphics[width=1\linewidth]{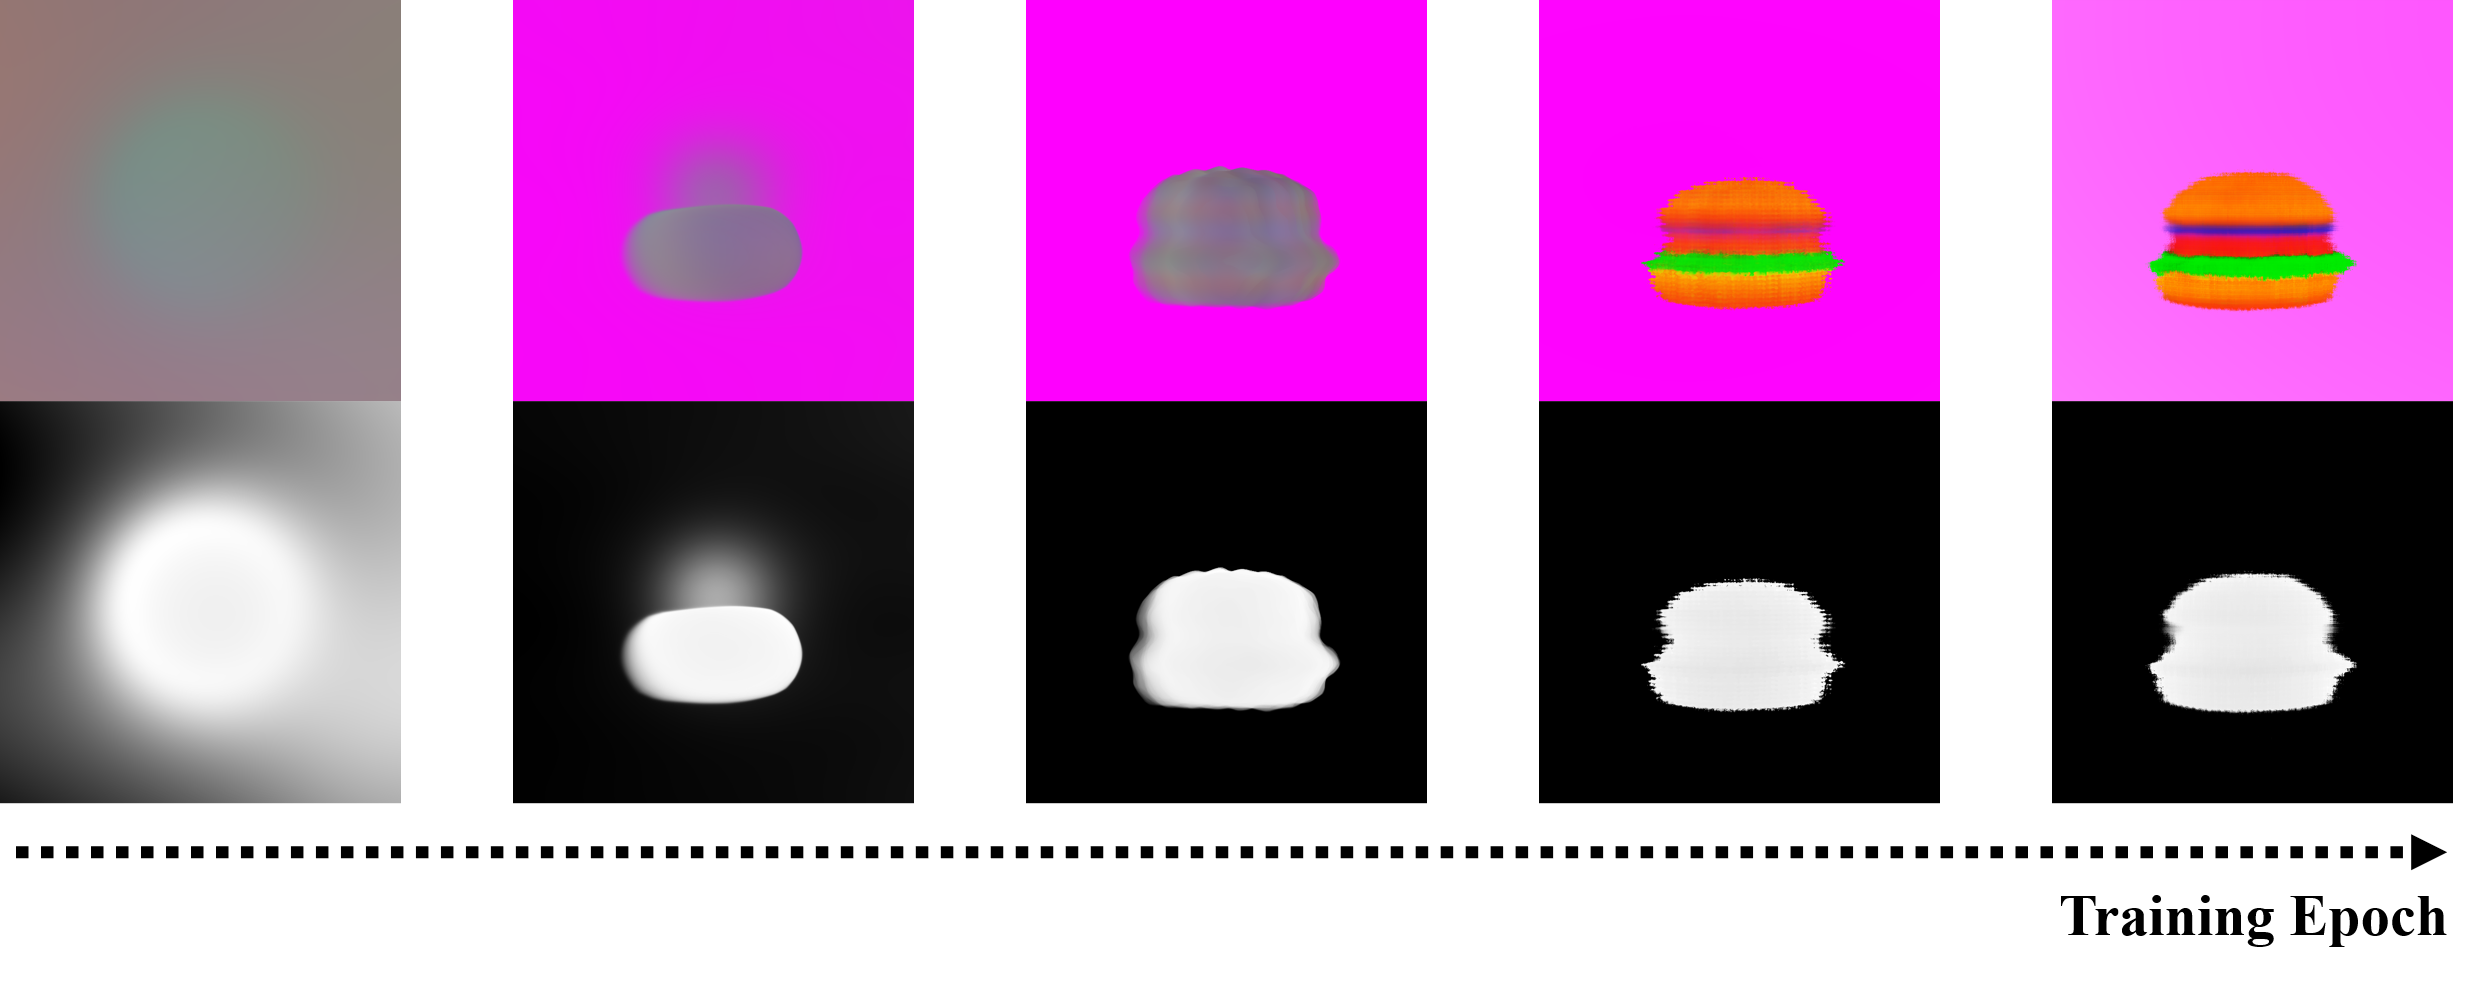}
    \caption{The training process of combining stable-dreamfusion with our proposed mi-MLP.}
    \end{subfigure}
    \caption{Given the input textual description, \ie, "a hamburger", (a) illustration of the training process of original stable-dreamfusion, (b) as well as the training process of modified stable-dreamfusion whose network structure is replaced by our proposed mi-MLP.}
    \label{fig:hamburger}
\end{figure}

\section{Additional Results on Few-shot View Synthesis}
\label{Additional Results on Few-shot View Synthesis}
As illustrated in Tab.~\ref{tab:suppl_blender}, Tab.~\ref{tab:suppl_llff} and Tab.~\ref{tab:suppl_shiny}, the additional quantitative results for each scene in the Blender, LLFF, and Shiny dataset are provided. We also show additional qualitative results of our proposed method in Fig.~\ref{fig:suppl_blender_4}, Fig.~\ref{fig:suppl_blender_8}, Fig.~\ref{fig:suppl_llff_3}, Fig.~\ref{fig:suppl_llff_6}, and Fig.~\ref{fig:suppl_llff_9}.

\begin{table*}
\centering
    \resizebox{0.8\linewidth}{!}{\begin{tabular}{c|ccccccccc}
    \toprule
    \multicolumn{10}{c}{\textbf{Blender-4}} \\
    \midrule
    Scene & \textbf{chair} & \textbf{drums} & \textbf{ficus} & \textbf{hotdog} & \textbf{lego} & \textbf{materials} & \textbf{mic} & \textbf{ship} & \textbf{Average} \\
    \midrule
    PSNR$\uparrow$  & 23.37 & 15.17 & 19.42 & 24.22 & 20.31 & 19.42 & 20.65 & 20.49 & 20.38 \\
    SSIM$\uparrow$  & 0.871 & 0.711 & 0.840  & 0.887 & 0.835 & 0.834 & 0.903 & 0.742 & 0.828 \\
    LPIPS$\downarrow$ & 0.121 & 0.258 & 0.129 & 0.121 & 0.160  & 0.124 & 0.109 & 0.238 & 0.157 \\
    Average$\downarrow$ & 0.058 & 0.161 & 0.083 & 0.053 & 0.084 & 0.083 & 0.066 & 0.102 & 0.084 \\
    \midrule
    \multicolumn{10}{c}{\textbf{Blender-8}} \\
    \midrule
    Scene & \textbf{chair} & \textbf{drums} & \textbf{ficus} & \textbf{hotdog} & \textbf{lego} & \textbf{materials} & \textbf{mic} & \textbf{ship} & \textbf{Average} \\
    \midrule
    PSNR$\uparrow$  & 27.75 & 19.85 & 21.49 & 29.85 & 25.50  & 22.33 & 27.15 & 23.69 & 24.70 \\
    SSIM$\uparrow$  & 0.936 & 0.844 & 0.876 & 0.948 & 0.887 & 0.864 & 0.949 & 0.777 & 0.885 \\
    LPIPS$\downarrow$ & 0.055 & 0.110  & 0.108 & 0.051 & 0.087 & 0.084 & 0.045 & 0.159 & 0.087 \\
    Average$\downarrow$ & 0.028 & 0.076 & 0.064 & 0.022 & 0.043 & 0.056 & 0.026 & 0.068 & 0.046 \\
    \bottomrule
    \end{tabular}%}
    \caption{The quantitative results for scenes in the Blender dataset with 4/8 input views available.
    }
    \label{tab:suppl_blender}
\end{table*}

\begin{table*}
\centering
    \resizebox{0.8\linewidth}{!}{\begin{tabular}{c|ccccccccc}
    \toprule
    \multicolumn{10}{c}{\textbf{LLFF-3}} \\
    \midrule
    Scene & \textbf{fern} & \textbf{flower} & \textbf{fortress} & \textbf{horns} & \textbf{leaves} & \textbf{orcids} & \textbf{room } & \textbf{trex} & \textbf{Average} \\
    \midrule
    PSNR$\uparrow$  & 21.43 & 19.61 & 23.38 & 17.40  & 16.42 & 15.70 & 23.17 & 20.86 & 19.75 \\
    SSIM$\uparrow$  & 0.675 & 0.580 & 0.580 & 0.486 & 0.494 & 0.470 & 0.880 & 0.741 & 0.614 \\
    LPIPS$\downarrow$ & 0.273 & 0.311 & 0.274 & 0.424 & 0.389 & 0.356 & 0.161 & 0.211 & 0.300 \\
    Average$\downarrow$ & 0.103 & 0.130 & 0.093 & 0.176 & 0.184 & 0.191 & 0.064 & 0.095 & 0.125 \\
    \midrule
    \multicolumn{10}{c}{\textbf{LLFF-6}} \\
    \midrule
    Scene & \textbf{fern} & \textbf{flower} & \textbf{fortress} & \textbf{horns} & \textbf{leaves} & \textbf{orcids} & \textbf{room } & \textbf{trex} & \textbf{Average} \\
    \midrule
    PSNR$\uparrow$  & 24.44 & 23.92 & 27.49 & 23.36 & 19.46 & 17.56 & 29.36 & 22.94 & 23.57 \\
    SSIM$\uparrow$  & 0.803 & 0.800 & 0.839 & 0.810 & 0.738 & 0.558 & 0.922 & 0.831 & 0.788 \\
    LPIPS$\downarrow$ & 0.164 & 0.130 & 0.116 & 0.179 & 0.177 & 0.280  & 0.098 & 0.164 & 0.163 \\
    Average$\downarrow$ & 0.063 & 0.061 & 0.043 & 0.071 & 0.100 & 0.148 & 0.031 & 0.069 & 0.069 \\
    \midrule
    \multicolumn{10}{c}{\textbf{LLFF-9}} \\
    \midrule
    Scene & \textbf{fern} & \textbf{flower} & \textbf{fortress} & \textbf{horns} & \textbf{leaves} & \textbf{orcids} & \textbf{room } & \textbf{trex} & \textbf{Average} \\
    \midrule
    PSNR$\uparrow$  & 25.89 & 25.94 & 29.26 & 25.37 & 20.95 & 18.50 & 29.93 & 25.33 & 25.15 \\
    SSIM$\uparrow$  & 0.846 & 0.854 & 0.883 & 0.862 & 0.788 & 0.615 & 0.934 & 0.889 & 0.834 \\
    LPIPS$\downarrow$ & 0.135 & 0.111 & 0.092 & 0.147 & 0.161 & 0.259 & 0.093 & 0.125 & 0.140 \\
    Average$\downarrow$ & 0.051 & 0.047 & 0.033 & 0.054 & 0.084 & 0.131 & 0.028 & 0.049 & 0.055 \\
    \bottomrule
    \end{tabular}%}
    \caption{The quantitative results for scenes in the LLFF dataset with 3/6/9 input views available.
    }
    \label{tab:suppl_llff}
\end{table*}

\begin{table*}
\centering
    \resizebox{0.8\linewidth}{!}{\begin{tabular}{c|ccccccccc}
    \toprule
    \multicolumn{10}{c}{\textbf{Shiny-3}} \\
    \midrule
    Scene & \textbf{cake} & \textbf{crest} & \textbf{food} & \textbf{giants} & \textbf{pasta} & \textbf{room} & \textbf{seasoning} & \textbf{tools} & \textbf{Average} \\
    \midrule
    PSNR$\uparrow$  & 20.41 & 14.31 & 16.06 & 18.98 & 14.78 & 22.37 & 19.78 & 19.28 & 18.24 \\
    SSIM$\uparrow$  & 0.439 & 0.251 & 0.353 & 0.509 & 0.442 & 0.569 & 0.506 & 0.730 & 0.475 \\
    LPIPS$\downarrow$ & 0.395 & 0.579 & 0.467 & 0.407 & 0.370 & 0.375 & 0.456 & 0.276 & 0.415 \\
    Average$\downarrow$ & 0.139 & 0.264 & 0.210 & 0.153 & 0.209 & 0.112 & 0.149 & 0.119 & 0.165 \\
    \bottomrule
    \end{tabular}%}
    \caption{The quantitative results for scenes in the Shiny dataset with 3 input views available.
    }
    \label{tab:suppl_shiny}
\end{table*}

\begin{figure*}
    \centering
    \includegraphics[width=0.9\linewidth]{figs/suppl_blender_4.png}
    \caption{The qualitative results for scenes in the Blender dataset with 4 input views available.}
    \label{fig:suppl_blender_4}
\end{figure*}

\begin{figure*}
    \centering
    \includegraphics[width=0.9\linewidth]{figs/suppl_blender_8.png}
    \caption{The qualitative results for scenes in the Blender dataset with 8 input views available.}
    \label{fig:suppl_blender_8}
\end{figure*}

\begin{figure*}
    \centering
    \includegraphics[width=0.9\linewidth]{figs/suppl_llff_3.png}
    \caption{The qualitative results for scenes in the LLFF dataset with 3 input views available.}
    \label{fig:suppl_llff_3}
\end{figure*}

\begin{figure*}
    \centering
    \includegraphics[width=0.9\linewidth]{figs/suppl_llff_6.png}
    \caption{The qualitative results for scenes in the LLFF dataset with 6 input views available.}
    \label{fig:suppl_llff_6}
\end{figure*}

\begin{figure*}
    \centering
    \includegraphics[width=0.9\linewidth]{figs/suppl_llff_9.png}
    \caption{The qualitative results for scenes in the LLFF dataset with 9 input views available.}
    \label{fig:suppl_llff_9}
\end{figure*}

\begin{figure*}
    \centering
    \includegraphics[width=0.9\linewidth]{figs/suppl_shiny_3.png}
    \caption{The qualitative results for scenes in the Shiny dataset with 3 input views available.}
    \label{fig:suppl_shiny_3}
\end{figure*}

\section{Limitations and Future Works}
\label{Limitations and Future Works}
Our proposed method aims to realize the task of few-shot view synthesis from the perspective of network structure, where state-of-the-art performance can be achieved. However, for objects with complex textures or thin structures, consistency across different views is hardly guaranteed since we impose no constraints on unknown novel views. To solve this problem, future works include introducing additional regularization terms or utilizing learned priors for better novel view synthesis.

% {
%     \small
%     \bibliographystyle{ieeenat_fullname}
%     \bibliography{supply}
% }
