# Supplementary material for: Is Vanilla MLP in Neural Radiance Field Enough for Few-shot View Synthesis?
Source: arXiv:2403.06092 source file (2024-03-10)
Supplement: Supplementary file 2 [file table_suppl_blender.tex]

\begin{tabular}{c|ccccccccc}
    \toprule
    \multicolumn{10}{c}{\textbf{Blender-4}} \\
    \midrule
    Scene & \textbf{chair} & \textbf{drums} & \textbf{ficus} & \textbf{hotdog} & \textbf{lego} & \textbf{materials} & \textbf{mic} & \textbf{ship} & \textbf{Average} \\
    \midrule
    PSNR$\uparrow$  & 23.37 & 15.17 & 19.42 & 24.22 & 20.31 & 19.42 & 20.65 & 20.49 & 20.38 \\
    SSIM$\uparrow$  & 0.871 & 0.711 & 0.840  & 0.887 & 0.835 & 0.834 & 0.903 & 0.742 & 0.828 \\
    LPIPS$\downarrow$ & 0.121 & 0.258 & 0.129 & 0.121 & 0.160  & 0.124 & 0.109 & 0.238 & 0.157 \\
    Average$\downarrow$ & 0.058 & 0.161 & 0.083 & 0.053 & 0.084 & 0.083 & 0.066 & 0.102 & 0.084 \\
    \midrule
    \multicolumn{10}{c}{\textbf{Blender-8}} \\
    \midrule
    Scene & \textbf{chair} & \textbf{drums} & \textbf{ficus} & \textbf{hotdog} & \textbf{lego} & \textbf{materials} & \textbf{mic} & \textbf{ship} & \textbf{Average} \\
    \midrule
    PSNR$\uparrow$  & 27.75 & 19.85 & 21.49 & 29.85 & 25.50  & 22.33 & 27.15 & 23.69 & 24.70 \\
    SSIM$\uparrow$  & 0.936 & 0.844 & 0.876 & 0.948 & 0.887 & 0.864 & 0.949 & 0.777 & 0.885 \\
    LPIPS$\downarrow$ & 0.055 & 0.110  & 0.108 & 0.051 & 0.087 & 0.084 & 0.045 & 0.159 & 0.087 \\
    Average$\downarrow$ & 0.028 & 0.076 & 0.064 & 0.022 & 0.043 & 0.056 & 0.026 & 0.068 & 0.046 \\
    \bottomrule
    \end{tabular}%
