# Supplementary material for: Is Vanilla MLP in Neural Radiance Field Enough for Few-shot View Synthesis?
Source: arXiv:2403.06092 source file (2024-03-10)
Supplement: Supplementary file 3 [file table_suppl_dropout.tex]

\begin{tabular}{c|cccc}
    \toprule
    Method & PSNR$\uparrow$  & SSIM$\uparrow$  & LPIPS$\downarrow$ & Average$\downarrow$ \\
    \midrule
    DietNeRF~\cite{jain2021putting} & \cellcolor{orange!25}23.83 & \cellcolor{yellow!25}0.859 & \cellcolor{yellow!25}0.117 & \cellcolor{yellow!25}0.056 \\
    Dropout~\cite{srivastava2014dropout} & \cellcolor{yellow!25}23.79 & \cellcolor{orange!25}0.875 & \cellcolor{orange!25}0.108 & \cellcolor{orange!25}0.054 \\
    mi-MLP (Ours) & \cellcolor{red!25}25.50  & \cellcolor{red!25}0.887 & \cellcolor{red!25}0.087 & \cellcolor{red!25}0.043 \\
    \bottomrule
    \end{tabular}%
