# Supplementary material for: Is Vanilla MLP in Neural Radiance Field Enough for Few-shot View Synthesis?
Source: arXiv:2403.06092 source file (2024-03-10)
Supplement: Supplementary file 4 [file table_suppl_llff.tex]

\begin{tabular}{c|ccccccccc}
    \toprule
    \multicolumn{10}{c}{\textbf{LLFF-3}} \\
    \midrule
    Scene & \textbf{fern} & \textbf{flower} & \textbf{fortress} & \textbf{horns} & \textbf{leaves} & \textbf{orcids} & \textbf{room } & \textbf{trex} & \textbf{Average} \\
    \midrule
    PSNR$\uparrow$  & 21.43 & 19.61 & 23.38 & 17.40  & 16.42 & 15.70 & 23.17 & 20.86 & 19.75 \\
    SSIM$\uparrow$  & 0.675 & 0.580 & 0.580 & 0.486 & 0.494 & 0.470 & 0.880 & 0.741 & 0.614 \\
    LPIPS$\downarrow$ & 0.273 & 0.311 & 0.274 & 0.424 & 0.389 & 0.356 & 0.161 & 0.211 & 0.300 \\
    Average$\downarrow$ & 0.103 & 0.130 & 0.093 & 0.176 & 0.184 & 0.191 & 0.064 & 0.095 & 0.125 \\
    \midrule
    \multicolumn{10}{c}{\textbf{LLFF-6}} \\
    \midrule
    Scene & \textbf{fern} & \textbf{flower} & \textbf{fortress} & \textbf{horns} & \textbf{leaves} & \textbf{orcids} & \textbf{room } & \textbf{trex} & \textbf{Average} \\
    \midrule
    PSNR$\uparrow$  & 24.44 & 23.92 & 27.49 & 23.36 & 19.46 & 17.56 & 29.36 & 22.94 & 23.57 \\
    SSIM$\uparrow$  & 0.803 & 0.800 & 0.839 & 0.810 & 0.738 & 0.558 & 0.922 & 0.831 & 0.788 \\
    LPIPS$\downarrow$ & 0.164 & 0.130 & 0.116 & 0.179 & 0.177 & 0.280  & 0.098 & 0.164 & 0.163 \\
    Average$\downarrow$ & 0.063 & 0.061 & 0.043 & 0.071 & 0.100 & 0.148 & 0.031 & 0.069 & 0.069 \\
    \midrule
    \multicolumn{10}{c}{\textbf{LLFF-9}} \\
    \midrule
    Scene & \textbf{fern} & \textbf{flower} & \textbf{fortress} & \textbf{horns} & \textbf{leaves} & \textbf{orcids} & \textbf{room } & \textbf{trex} & \textbf{Average} \\
    \midrule
    PSNR$\uparrow$  & 25.89 & 25.94 & 29.26 & 25.37 & 20.95 & 18.50 & 29.93 & 25.33 & 25.15 \\
    SSIM$\uparrow$  & 0.846 & 0.854 & 0.883 & 0.862 & 0.788 & 0.615 & 0.934 & 0.889 & 0.834 \\
    LPIPS$\downarrow$ & 0.135 & 0.111 & 0.092 & 0.147 & 0.161 & 0.259 & 0.093 & 0.125 & 0.140 \\
    Average$\downarrow$ & 0.051 & 0.047 & 0.033 & 0.054 & 0.084 & 0.131 & 0.028 & 0.049 & 0.055 \\
    \bottomrule
    \end{tabular}%
