# Supplementary material for: Is Vanilla MLP in Neural Radiance Field Enough for Few-shot View Synthesis?
Source: arXiv:2403.06092 source file (2024-03-10)
Supplement: Supplementary file 5 [file table_suppl_shiny.tex]

\begin{tabular}{c|ccccccccc}
    \toprule
    \multicolumn{10}{c}{\textbf{Shiny-3}} \\
    \midrule
    Scene & \textbf{cake} & \textbf{crest} & \textbf{food} & \textbf{giants} & \textbf{pasta} & \textbf{room} & \textbf{seasoning} & \textbf{tools} & \textbf{Average} \\
    \midrule
    PSNR$\uparrow$  & 20.41 & 14.31 & 16.06 & 18.98 & 14.78 & 22.37 & 19.78 & 19.28 & 18.24 \\
    SSIM$\uparrow$  & 0.439 & 0.251 & 0.353 & 0.509 & 0.442 & 0.569 & 0.506 & 0.730 & 0.475 \\
    LPIPS$\downarrow$ & 0.395 & 0.579 & 0.467 & 0.407 & 0.370 & 0.375 & 0.456 & 0.276 & 0.415 \\
    Average$\downarrow$ & 0.139 & 0.264 & 0.210 & 0.153 & 0.209 & 0.112 & 0.149 & 0.119 & 0.165 \\
    \bottomrule
    \end{tabular}%
